# Supplementary material for: Strengthening gold-gold bonds by complexing gold clusters with noble gases
Source: arXiv:1503.03750 ancillary file (2015-03-12)
Supplement: Supplementary file 1 [file AuKr_SI.pdf]

Strengthening gold-gold bonds  
by complexing gold clusters with noble gases  
Luca M. Ghiringhelli and Sergey V. Levchenko

SUPPLEMENTARY MATERIAL

**Computational details**

The theoretical results presented in this work were obtained using the FHI-aims [1] program package for an accurate all-electron description based on numeric atom-centered basis functions. The IR spectra at finite temperature were calculated by performing Born-Oppenheimer molecular dynamics (MD) simulations in the *canonical* ensemble and extracting from the trajectories the Fourier transform of the dipole-dipole autocorrelation function. The IR intensities are then computed via:

$$I(\omega) \propto \beta \omega^2 \int_0^\infty dt \left\langle \vec{M}(t) \cdot \vec{M}(0) \right\rangle_{NVT} \exp(i\omega t) \quad (1)$$

where  $\vec{M}(t)$ , is the total electric dipole of the cluster at time  $t$ ,  $\beta = 1/kT$  and the angular brackets indicate an ensemble average in the canonical ensemble. We assume the system as ergodic: This means that a time average performed on a long thermostatted trajectory is equivalent to an ensemble average in the  $NVT$  ensemble. A trajectory is judged “long enough” when the vibrational spectrum calculated for the whole trajectory does not change any more. The energy and forces for MD are calculated with (collinear) spin-polarized DFT at the PBE [2] generalized gradient approximation level, corrected for long range vdW interactions via the Tkatchenko-Scheffler (TS) scheme, *i.e.* a sum over  $C_6[n]/R^6$  tails with  $C_6$  coefficients derived from the self-consistent electron density  $n$  and reference values for the free atoms [3]. This functional is referred throughout the paper as PBE+vdW. We used “really tight” integration grid settings and accurate “tier 2” basis sets [1]. The “scaled ZORA” scalar relativistic correction [4], as implemented in FHI-aims [1] was used

The performance of PBE+vdW for geometries and binding energies is validated for  $\text{Au}_2$  and  $\text{Au}_2\cdot\text{Kr}$  by PBE0+vdW (PBE0 [5] with TS vdW correction) and B3LYP [6] hybrid functionals, XYG3 doubly hybrid functional [7], renormalized second-order perturbation

theory (rPT2) [8], MP2, and CCSD(T). For benchmarking, we also compared the M06-2X functional [9] to the above methods. The molecular orbitals of  $\text{Au}_M\text{Kr}_N$  clusters were also calculated with  $G_0W_0\text{@PBE0}$  and self-consistent  $GW$  (sc- $GW$ ), as implemented in FHI-aims [10, 11]. CCSD(T) calculations were performed using Gaussian03 code [12] with aug-cc-pVTZ-PP basis set of Peterson and Puzzarini [13, 14, 15].

Harmonic vibrational frequencies and intensities were computed from finite differences of the analytic forces. For the MD, we used “tight” integration grid settings and “tier 2” basis sets, and the “atomic ZORA” scalar relativistic correction [1]. The assessment on the convergence of the settings is presented elsewhere [16]. The electronic structure was computed using fully-converged integration grids and basis sets.

- [1] Blum, V.; Gehrke, R.; Hanke, F.; Havu, P.; Havu, V.; Ren, X.; Reuter, K.; Scheffler, M. *Comp. Phys. Comm.* 2009, *180*, 2175.
- [2] Perdew, J. P.; Burke, K.; Ernzerhof, M. *Phys. Rev. Lett.* 1996, *77*, 3865.
- [3] Tkatchenko, A.; Scheffler, M. *Phys. Rev. Lett.* 2009, *102*, 6.
- [4] van Lenthe, E.; Baerends, E. J.; Snijders, J. G. *J. Chem. Phys.* 1994, *101*, 9783.
- [5] Adamo, C.; Barone, V. *J. Chem. Phys.* 1999, *110*, 6158.
- [6] Lee, C.; Yang, W.; Parr, R. G. *Phys. Rev. B* 1988, *37*, 785. Becke, A.D. *Phys. Rev. A* 1988, *38*, 3098. Becke, A.D. *J. Chem. Phys.* 1993, *98*, 5648.
- [7] Zhang, Y.; Xua, X.; Goddard III, W. A. *Proc. Natl. Acad. Sci. USA* 2008, *106*, 4963.
- [8] Ren, X.; Rinke, P.; Joas, C.; Scheffler, M. *J. Mater. Sci.* 2012, *47*, 7447.
- [9] Zhao, Y.; Truhlar, D. G. *Theor. Chem. Acc.* 2008, *120*, 215.
- [10] Ren, X.; Rinke, P.; Blum, V.; Wieferink, J.; Tkatchenko, A.; Sanfilippo, A.; Reuter, K.; Scheffler, M. *New J. Phys.* 2012, *14*, 053200.
- [11] Caruso, F.; Rinke, P.; Ren, X.; Scheffler, M.; Rubio, A. *Phys. Rev. B* 2012, *86*, 081102(R).
- [12] Frisch, M. J. et al. *Gaussian 03, Revision D.01*, Gaussian, Inc., Wallingford, CT, 2004.
- [13] Figgen, D.; Rauhut, G.; Dolg, M.; Stoll, H. *Chem. Phys.* 2005, *311*, 227.
- [14] Peterson, K.; C., P. *Theor. Chem. Acc.* 2005, *114*, 283.
- [15] Peterson, K.; Figgen, D.; Goll, E.; Stoll, H.; Dolg, M. *J. Chem. Phys.* 2003, *119*, 11113.
- [16] Ghiringhelli, L. M.; Gruene, P.; Lyon, J. T.; Meijer, G.; Fielicke, A.; Scheffler, M. *New J. Phys.* 2013, *15*, 083003.

# Structural and vibrational parameters

| Molecule                         | bond<br>[Å] | $\Delta$ bond<br>[Å] | % $\Delta$ bond | vib. freq.<br>[cm <sup>-1</sup> ] | $\Delta$ vib. freq.<br>[cm <sup>-1</sup> ] | % $\Delta$ vib. freq. |
|----------------------------------|-------------|----------------------|-----------------|-----------------------------------|--------------------------------------------|-----------------------|
| Au <sub>2</sub>                  | 2.527       |                      |                 | 173.1                             |                                            |                       |
| Au <sub>2</sub> <sup>-</sup>     | 2.632       |                      |                 | 132.1                             |                                            |                       |
| Au <sub>2</sub> ·Kr              | 2.520       | -0.007               | -0.27           | 181.4                             | 8.4                                        | 4.8                   |
| Au <sub>2</sub> ·Kr <sub>2</sub> | 2.515       | -0.012               | -0.47           | 187.1                             | 14.0                                       | 8.1                   |
| Au <sub>3</sub>                  | 2.616       |                      |                 | 59.0                              | bending (stretch long bond)                |                       |
|                                  | 2.616       |                      |                 | 99.7                              | asymm. stretch                             |                       |
|                                  | 2.879       |                      |                 | 162.7                             | symm.stretch                               |                       |
| Au <sub>3</sub> <sup>-</sup>     | 2.720       |                      |                 | 88.0                              | asymm. stretch                             |                       |
|                                  | 2.720       |                      |                 | 88.1                              | bending                                    |                       |
|                                  | 2.720       |                      |                 | 139.4                             | symm.stretch                               |                       |
| Au <sub>3</sub> ·Kr              | 2.626       | 0.010                | 0.4             | 75.8                              | 16.8                                       | 28.5                  |
|                                  | 2.626       | 0.010                | 0.4             | 100.6                             | 1.1                                        | 1.1                   |
|                                  | 2.804       | -0.075               | -2.6            | 166.3                             | 3.6                                        | 2.2                   |
| Au <sub>3</sub> ·Kr <sub>2</sub> | 2.751       | 0.135                | 5.2             | 105.9                             | 46.9                                       | 79.5                  |
|                                  | 2.751       | 0.135                | 5.2             | 74.7                              | -25.0                                      | -25.1                 |
|                                  | 2.562       | -0.318               | -11.0           | 176.9                             | 14.2                                       | 8.7                   |

TABLE I. Structural parameters and harmonic vibrational frequencies with PBE+vdW of the structures discussed in the text. Note that, for Au<sub>3</sub>Kr<sub>2</sub>, the frequencies of invert, i.e. the mode at 105.9 cm<sup>-1</sup> is a bending (stretching of the short bond), while the mode at 74.7 is the asymmetric stretch (Kr is rather fix in both these modes). This is consistent with the fact that the long Au-Au bond shortens by 11%.

## Hirshfeld and Mulliken partitioning

| Molecule                          | Atom    | H charge [ $e^-$ ] | M charge [ $e^-$ ] | M population                    |
|-----------------------------------|---------|--------------------|--------------------|---------------------------------|
| $\text{Au}_2\cdot\text{Kr}$       | far Au  | -0.07              | -0.07              | $6s^{0.10}6p^{0.00}5d^{-0.02}$  |
|                                   | near Au | -0.06              | -0.04              | $6s^{-0.01}6p^{0.10}5d^{-0.06}$ |
|                                   | Kr      | 0.13               | 0.11               | $4p^{-0.14}3d^{0.03}$           |
| $\text{Au}_2\cdot\text{Xe}$       | far Au  | -0.10              | -0.12              | $6s^{0.14}6p^{0.00}5d^{0.03}$   |
|                                   | near Au | -0.07              | -0.05              | $6s^{-0.04}6p^{0.15}5d^{-0.08}$ |
|                                   | Xe      | 0.17               | 0.17               | $5p^{-0.22}4d^{0.05}$           |
| $\text{AuXe}^+$ [1]               | Au      |                    | -0.39              | $6s^{0.29}6p^{0.12}5d^{-0.05}$  |
|                                   | Xe      |                    | 0.39               | $5p^{-0.49}4d^{0.10}$           |
| $\text{Au}_2\cdot\text{Kr}_2$     | both Au | -0.11              | -0.11              | $6s^{0.07}6p^{0.10}5d^{-0.07}$  |
|                                   | both Kr | 0.11               | 0.11               | $4p^{-0.14}3d^{0.03}$           |
| $\text{Au}\cdot\text{Kr}_2^+$ [1] | Au      |                    | 0.35               | $6s^{0.51}6p^{0.21}5d^{-0.11}$  |
|                                   | both Kr |                    | -0.35              | $4p^{-0.45}3d^{0.10}$           |

TABLE II. Comparison of partial charges and population analysis for selected clusters. Hirshfeld partial charge (H) is with the converged “tier 2” basis set. Mulliken (M) partial charge and population is with a less diffuse “tier 1 –  $\{gh\}$ ” basis set.

[1] Pyykkö, P. *J. Am. Chem. Soc.* **1995**, **117**, 20672070

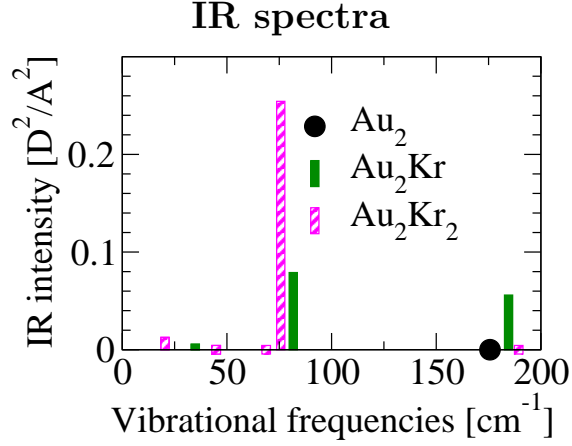

FIG. 1. IR spectrum of  $\text{Au}_2\text{Kr}_2$  and  $\text{Au}_2\text{Kr}$ , compared to the pristine  $\text{Au}_2$  dimer. The symbols crossing the x-axis are IR-inactive modes and they are reported in order to show the trends in their frequency value.

### DoS for the binding of various rare gas atoms to $\text{Au}_2$

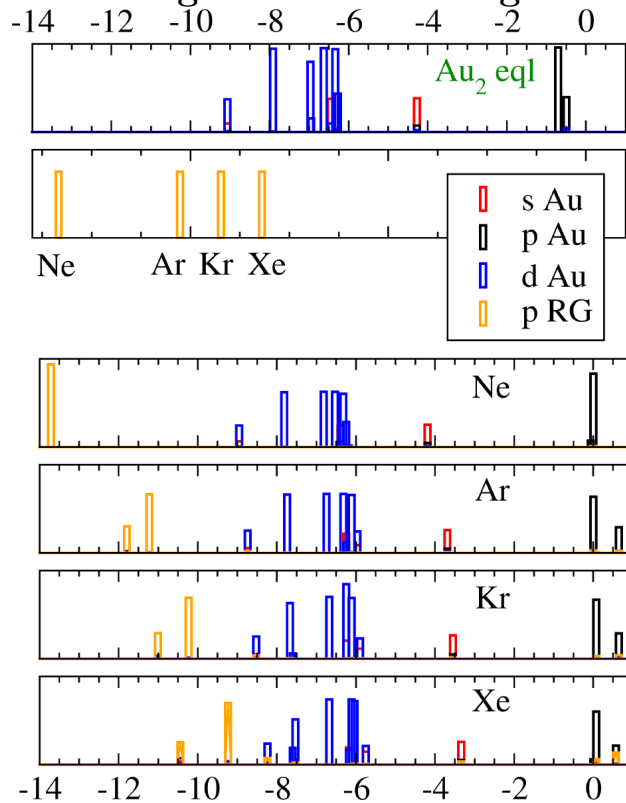

FIG. 2. Electronic density of states picture of the adsorption of Ne, Ar, Kr, and Xe on  $\text{Au}_2$ . The overlap between  $p$  valence orbitals of the rare gases and  $\delta_{z^2}$  molecular orbital of  $\text{Au}_2$  is maximized for Kr.

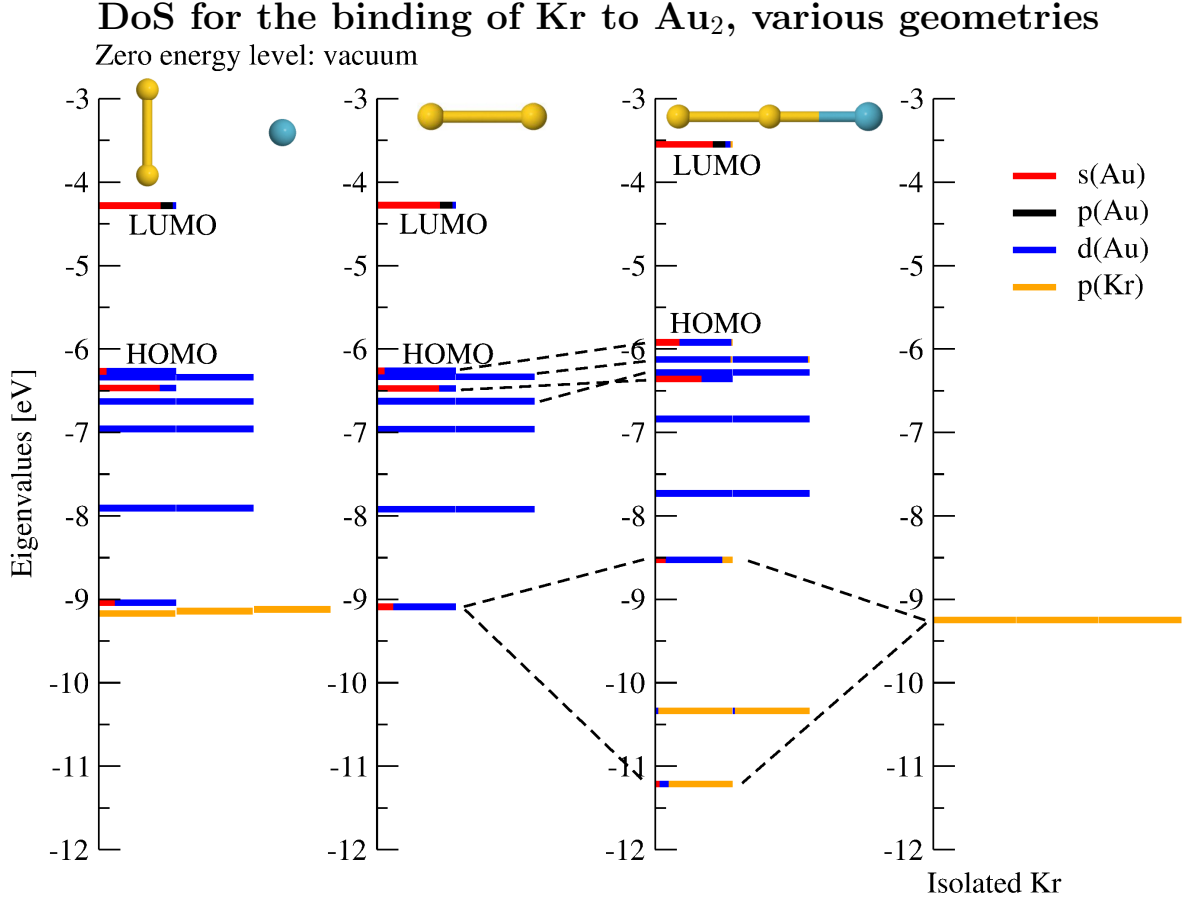

FIG. 3. Molecular orbital picture of Kr bonding to gold dimer, based on atom and angular momentum projected electronic (KS) DoS. All structures are calculated at really-tight settings, tier 2 basis set, and PBE+vdW functional. When Kr is adsorbed on the dimer forming a linear Au<sub>2</sub>Kr molecule, its  $p$  orbitals split and  $p_z$  hybridizes with the  $\sigma(s - d_{z^2})$  orbital of Au<sub>2</sub>. A complex redistribution of  $d$  and  $sd$  orbitals is also evident. When Kr is in the “bridge” equilibrium position, Au<sub>2</sub> orbitals are hardly perturbed. Kr  $p$  orbitals show a fine splitting (smaller than the thickness of the bar) due to symmetry breaking and very weak long-range interaction with the dimer. The zero energy level is vacuum.

# DoS for the binding of Kr to Au<sub>2</sub>, PBE, PBE0, and $G_0W_0$ @PBE0

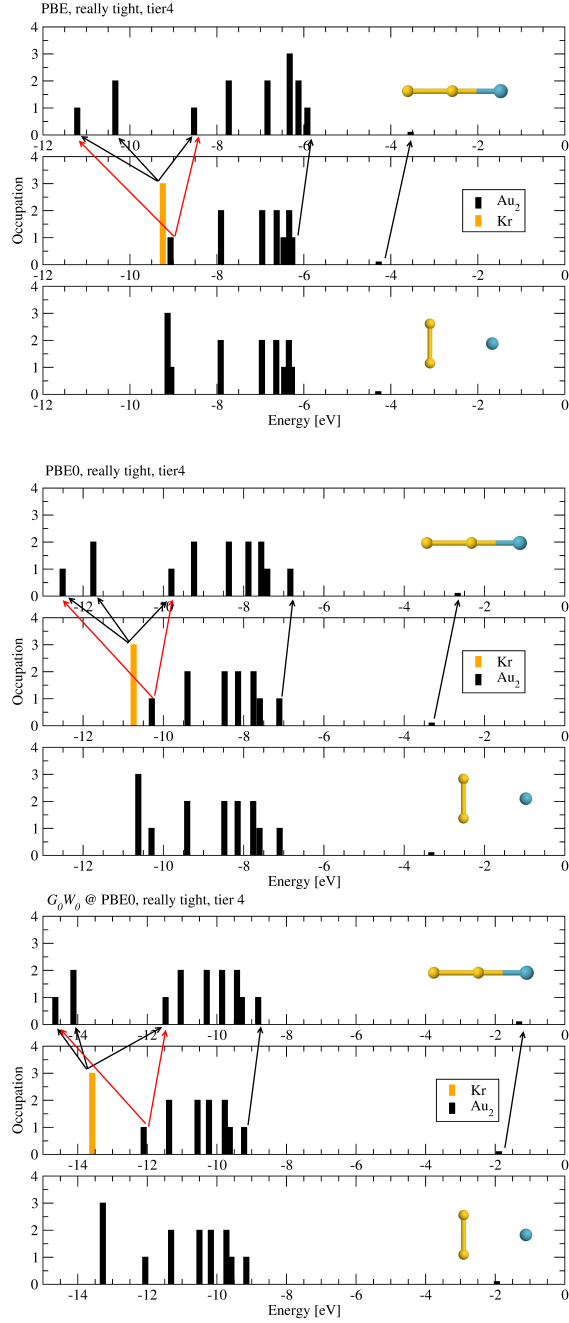

FIG. 4. Electronic (KS) DoS obtained with (from top) PBE, PBE0, and  $G_0W_0$ @PBE0 functionals (really tight, tier 4, all cases). In each plot the top panel is for the linear Kr@Au<sub>2</sub> molecule, the center panel for the isolated dimer and Kr atom, the bottom panel for the bridge Kr@Au<sub>2</sub>. The arrows mark the interpretation of Kr *p*-orbital splitting and mixing of *p<sub>z</sub>* with the  $\sigma(s-d_{z^2})$  orbital of Au<sub>2</sub>, when the linear Kr@Au<sub>2</sub> is formed. For PBE and PBE0, this interpretation is supported by the atom and angular momentum projected DoS. For  $G_0W_0$ @PBE0, this is done by analogy. For bridge Kr@Au<sub>2</sub> Au<sub>2</sub> and Kr orbitals are hardly perturbed, in all cases. The zero energy level is vacuum.

## DoS for the binding of Kr to Au<sub>2</sub>, self-consistent *GW*

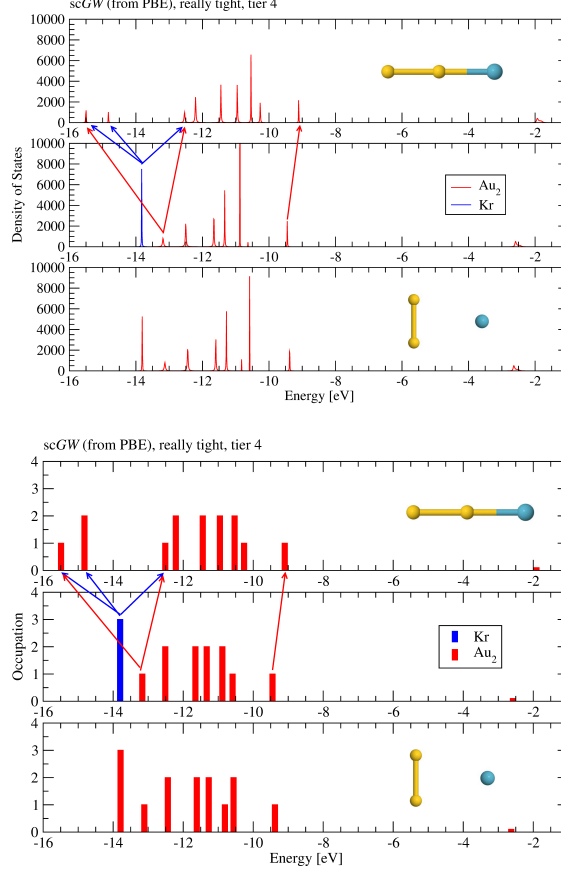

FIG. 5. Electronic (KS) DoS obtained with self-consistent *GW* (sc*GW*) starting from PBE orbitals. The bottom plot is a “coarse grained” version of the sc*GW* spectrum, drawn in order to facilitate the comparison to the other methods. It was obtained from the continuous spectrum by assigning the integral under each peak at the position of the baricenter of the peak. In each plot the top panel is for the linear Au<sub>2</sub>-Kr molecule, the center panel for the isolated gold dimer and Kr atom, the bottom panel for the bridge (triangular) Au<sub>2</sub>-Kr. The arrows mark the interpretation of Kr *p*-orbital splitting and mixing of *p<sub>z</sub>* with the  $\sigma(s - d_{z^2})$  orbital of Au<sub>2</sub>, when the linear Au<sub>2</sub>-Kr is formed. As for  $G_0W_0$ @PBE0, this is done by analogy to PBE and PBE0 projected orbitals. For bridge Au<sub>2</sub>-Kr, Au<sub>2</sub> and Kr orbitals are hardly perturbed. The zero energy level is vacuum.

## Contour plots of electron-density differences upon Kr adsorption

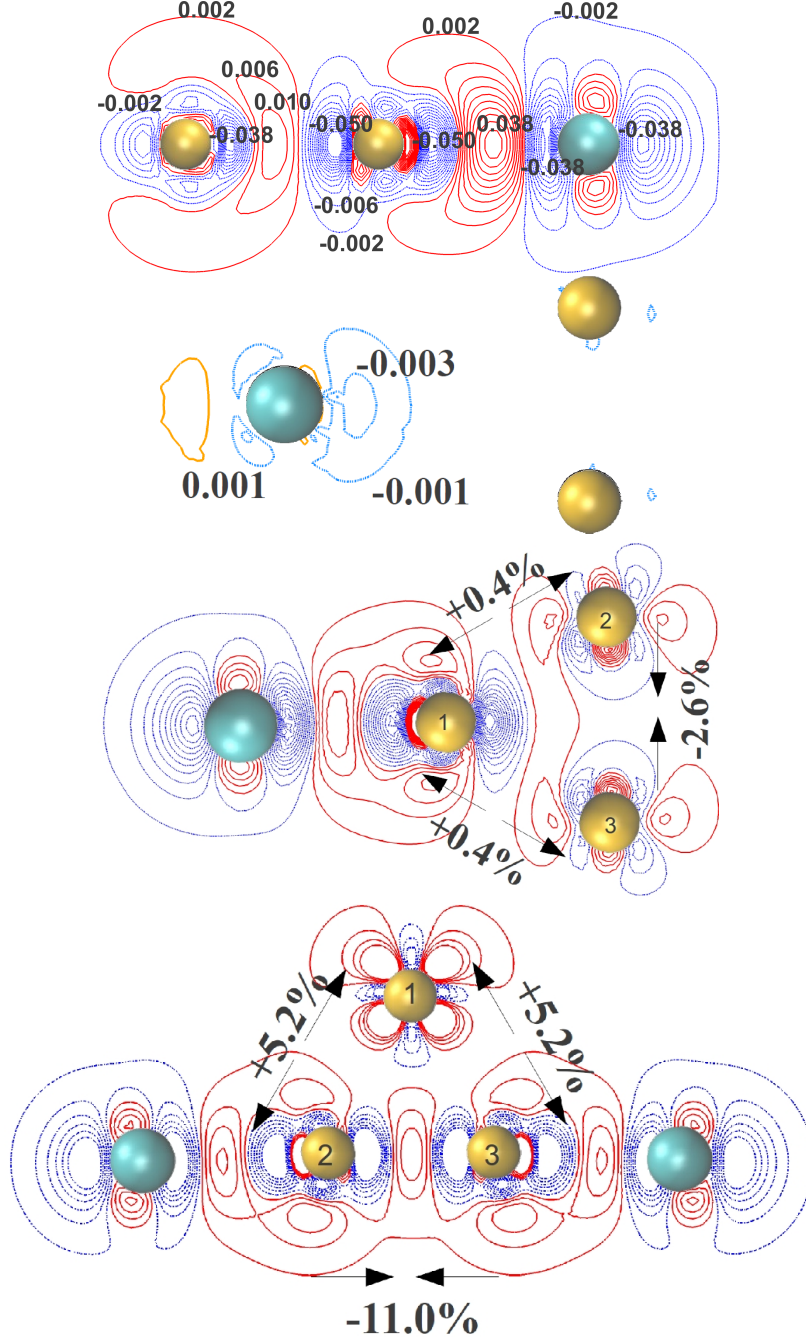

FIG. 6. Contour plots of the electron density difference for various  $\text{Au}_M \cdot \text{Kr}_N$ , i.e.  $n(\text{Au}_M \cdot \text{Kr}_N) - n(\text{Au}_M) - Nn(\text{Kr})$ . For  $\text{Au}_3 \cdot \text{Kr}_N$  also the relative amount and direction of the bond length changes upon Kr adsorption are indicated. The isolevels are the same in all plots, i.e., the most external line is at  $\pm 0.002e^-/\text{\AA}^3$  and the space between lines is  $0.004e^-/\text{\AA}^3$ . Yellow (blue) circles represent Au (Kr) nuclei. The numbers inside the circles representing the gold atoms are used in the text for indicating a particular gold atom.

# Kohn-Sham Molecular Orbitals picture of Kr adsorbing on $\text{Au}_3$

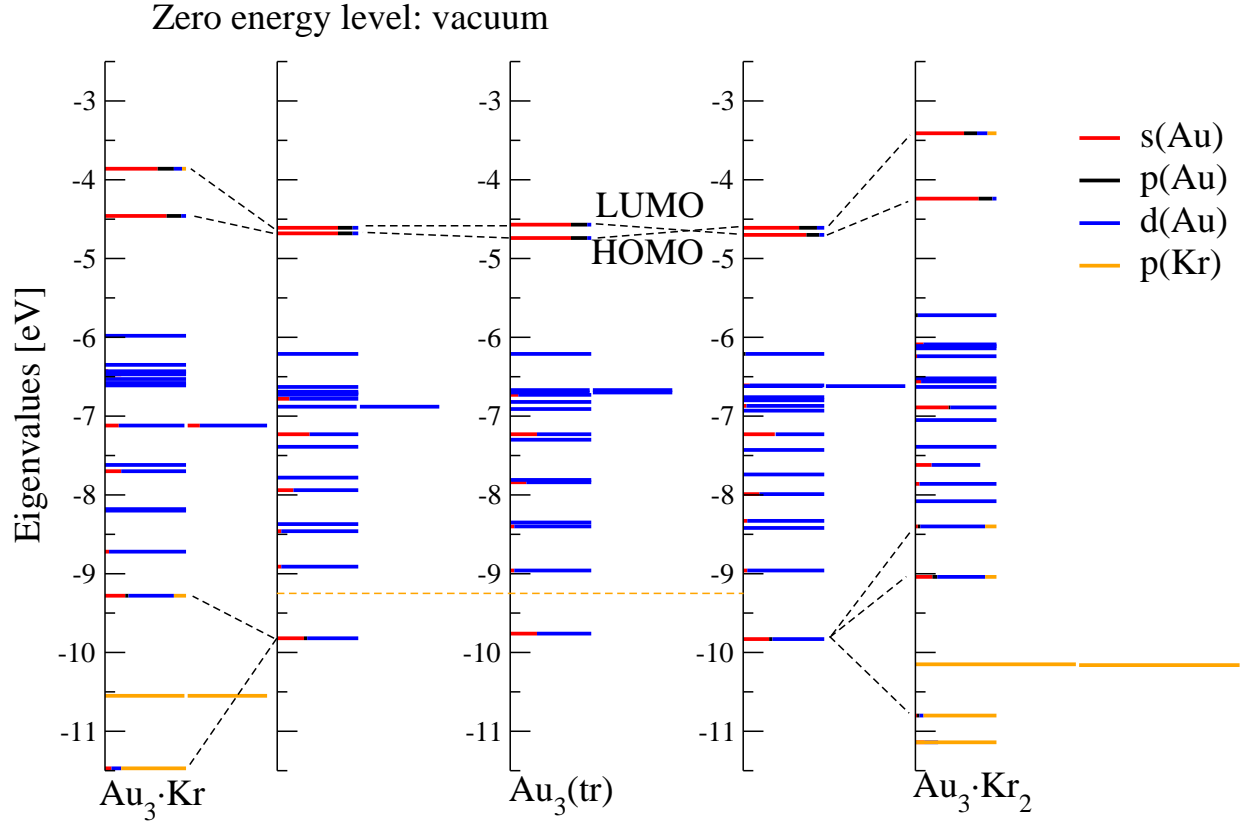

FIG. 7. Molecular orbital picture of Kr bonding to gold (acuteangle) trimer. The dashed orange (horizontal) line marks the level of the  $p$  orbitals of isolated Kr wrt vacuum. The black dashed lines are guides for the eyes linking similar orbitals in different molecular arrangements. Starting from the center column, where we show the relaxed acute-angled trimer, and going to the left, one finds  $\text{Au}_3$  in the geometry of  $\text{Au}_3 \cdot \text{Kr}$  and then the relaxed  $\text{Au}_3 \cdot \text{Kr}$ . Going to the right one finds  $\text{Au}_3$  in the geometry of  $\text{Au}_3 \cdot \text{Kr}_2$  and then the relaxed  $\text{Au}_3 \cdot \text{Kr}_2$ .
